# Supplementary material for: Predicting passenger loading level on a train car: A Bayesian approach
Source: arXiv:1808.06962 source file (2018-08-01)
Supplement: Supplementary file 1 [file appendix.tex]

\appendix
\section{Multi-DOF model of train carbody vibrations}
\label{appendix:multi_dof}
In \cite{zhou2009influences} authors model a train carbody as a simple uniform Euler-Bernouli beam. This is a half-car model, i.e. only a half of the train car is considered with two bogies and a pair of wheels at each bogie. The carbody of mass, $m_b$, and length, $L$, is supported by a set of secondary suspensions with spring stiffness, $k_s$, and damping coefficient, $c_s$, per bogie as shown in Figure \ref{fig:mdof_model}. The secondary suspensions are attached to the bogies which are modeled as solid (non-flexible) bodies with equal masses, $m_t$. Bogies can only experience bounce and pitch displacements. A pair of wheels is attached to each bogie through primary suspension with spring stiffness and damping coefficient, $k_p$, and, $c_p$, respectively. It is assumed that the wheels cannot jump. Thus, wheels can only move up and down in correspondence to the irregularities in the rail track. From the beam theory the equation for Euler-Bernouli beam deflections is
\begin{equation}
\label{eq:euler_bernouili}
EI \dfrac{ \partial^4 z(x,t)}{\partial x^4} + \mu I \frac{\partial^5 z(x,t)}{\partial t \partial x^4} + \rho \frac{\partial ^ 2 z(x,t)}{\partial t^2} = P_1 \delta(x-l_1) + P_2\delta(x-l_2),
\end{equation}
where 
$E$ is an elastic modulus of the carbody, $I$ is an equivalent beam moment of inertia, $\mu$ is a structural damping coefficient, $\rho = m_b/L$ is a mass per unit length, $z(x,t)$ is a carbody displacement at the location $x$ and time $t$,
$P_1$ and $P_2$ are the forces acted by the secondary suspension on the carbody at positions $l_1$ and $l_2$ respectively (Figure \ref{fig:mdof_model})
\begin{eqnarray}
\label{eq:force1}
P_1 = -k_s[z(l_1, t) - z_{t1}] - c_s[\dot{z}(l_1,t)-\dot{z}_{t1}],\\
\label{eq:force2}
P_2 = -k_s[z(l_2, t) - z_{t2}] - c_s[\dot{z}(l_2,t)-\dot{z}_{t2}],
\end{eqnarray}
and $z_{t1}$ and $z_{t2}$ are the vertical displacements of the bogies.

The partial differential equation in (\ref{eq:euler_bernouili}) can be solved by using the variables separation method. The carbody deflections, $z(x,t)$, can be represented using functions, $Y_i(x)$, that describe spatial shapes of the deflection modes and thus depend only on the spatial coordinate $x$, and functions, $q_i(t)$, known as modal coordinates, that describe temporal variations and depend only on time variable $t$
\begin{equation}
\label{eq:displacement}
z(x,t) = z_b(t) + \left(\frac{L}{2} - x \right)\theta_b(t) + \sum_{i=3}^n Y_i(x)q_i(t),
\end{equation}
here $z_b(t)$ denotes the bounce rigid mode of the carbody (i.e. $q_1(t) = z_b(t)$ and $Y_1(x) = 1$ ), $\theta_b(t)$ is the carbody pitch angle ($q_2(t) = \theta_b(t)$ and $Y_2(x) = L/2 - x$), and $n$ is total number of the considered modes. It can be shown that the higher order ($i>2$) modes are the flexible modes that have the following spatial shapes
\begin{equation}
Y_i(x) = \cosh\beta_ix+\cos\beta_ix - \frac{\cosh\lambda_i - \cos\lambda_i}{\sinh\lambda_i - \sin\lambda_i}\left(\sinh\beta_ix + \sin\beta_ix\right),
\end{equation}
where $\lambda_i$ and $\beta_i$ must satisfy
\begin{eqnarray}
1-\cosh\lambda_i\cos\lambda_i = 0 \textrm{, } \beta_i = \frac{\lambda_i}{L}.
\end{eqnarray}
Solutions for modal coordinates, $q_i(t)$, can be obtained by substituting (\ref{eq:displacement}) into (\ref{eq:euler_bernouili}) and integrating along the lengths of the carbody in order to eliminate the spatial variable $x$. Since the modal shape functions, $Y_i(x)$, are orthogonal to each other for different $i$, we obtain
\begin{align}
\label{eq:carbody_modes1}
m_b&\ddot{z}_b(t) =P_1+P_2,\\
I_b&\ddot{\theta}_b(t) =P_1\left(\frac{L}{2}-l_1\right)+P_2\left(\frac{L}{2}-l_2\right),\\
\ddot{q}_i&(t)  +\frac{\mu I \beta_i^4}{\rho}\dot{q_i(t)} + \frac{EI\beta_i^4}{\rho}q_i(t) = \frac{Y_i(l_1)}{m_b}P_1 + \frac{Y_i(l_2)}{m_b}P_2, i=3,4,\ldots,n \label{eq:higher_order_modes}
\end{align}
were $I_b$ is the carbody pitch inertia.

Equation (\ref{eq:higher_order_modes}) is a second order differential equation that describes a driven harmonic oscillator (a second order system). Hence this equation for the $i^{\rm th}$ mode can be rewritten in terms of the natural frequency, $\omega_i$, and the damping ratio, $\xi_i$, of the corresponding harmonic oscillator
\begin{equation}
\ddot{q}_i(t) +2\xi_i\omega_i\dot{q_i(t)} + \omega_i^2q_i(t) = \frac{Y_i(l_1)}{m_b}P_1 + \frac{Y_i(l_2)}{m_b}P_2 \textrm{, } i=3,4,\ldots,n 
\end{equation}
where 
\begin{equation}
\omega_i^2 = \frac{EI\beta_i^4}{\rho}\textrm{, } \xi_i = \frac{\mu I \beta_i^4}{2\rho\omega_i}.
\end{equation}
Further, the forces in (\ref{eq:force1}) and (\ref{eq:force2}) can be rewritten using (\ref{eq:displacement}) as
\begin{align}
\label{eq:force1_2}
P_1 = & -k_s\left[z_b(t)+\left(\frac{L}{2}-l_1\right)\theta_b(t) + \sum_{i=3}^n Y_i(l_1)q_i(t)-z_{t1}\right]\nonumber\\
&-c_s\left[\dot{z}_b(t) + \left(\frac{L}{2}-l_1\right)\dot{\theta}_b(t) + \sum_{i=3}^n Y_i(l_1)\dot{q}_i(t) - \dot{z}_{t1}\right],\\
\label{eq:force2_2}
P_2 = & -k_s\left[z_b(t)+\left(\frac{L}{2}-l_2\right)\theta_b(t) + \sum_{i=3}^n Y_i(l_2)q_i(t)-z_{t2}\right]\nonumber\\
&-c_s\left[\dot{z}_b(t) + \left(\frac{L}{2}-l_2\right)\dot{\theta}_b(t) + \sum_{i=3}^n Y_i(l_2)\dot{q}_i(t) - \dot{z}_{t2}\right].
\end{align}

The equations for bogie bounce and pitch follow from Newton's second law
\begin{align}
\label{eq:bogie1}
m_t\ddot{z}_{t1} =& -k_s(z_{t1}-z(l_1,t))-c_s(\dot{z}_{t1}-\dot{z}(l_1,t))-k_p(z_{t1}-l_w\theta_{t1}-z_{w1}) \nonumber\\
&-c_p(\dot{z}_{t1}-l_w\dot{\theta}_{t1}-\dot{z}_{w1}) -k_p(z_{t1}+l_w\theta_{t1}-z_{w2})-c_p(\dot{z}_{t1}+l_w\dot{\theta}_{t1}-\dot{z}_{w2}),\\
I_t\ddot{\theta}_{t1} =&l_wk_p(z_{t1}-l_w\theta_{t1}-z_{w1}) + l_w c_p(\dot{z}_{t1}-l_w\dot{\theta}_{t1}-\dot{z}_{w1} ) \nonumber \\
&-l_w k_p(z_{t1}+l_w\theta_{t1}-z_{w2})-l_w c_p(\dot{z}_{t1}+l_w\dot{\theta}_{t1}-\dot{z}_{w2}),\\
m_t\ddot{z}_{t2} =& -k_s(z_{t2}-z(l_2,t))-c_s(\dot{z}_{t2}-\dot{z}(l_2,t))-k_p(z_{t2}-l_w\theta_{t2}-z_{w3}) \nonumber\\
&-c_p(\dot{z}_{t2}-l_w\dot{\theta}_{t2}-\dot{z}_{w3}) -k_p(z_{t2}+l_w\theta_{t2}-z_{w4})-c_p(\dot{z}_{t2}+l_w\dot{\theta}_{t2}-\dot{z}_{w4}),\\
I_t\ddot{\theta}_{t2} =&l_wk_p(z_{t2}-l_w\theta_{t2}-z_{w3}) + l_w c_p(\dot{z}_{t2}-l_w\dot{\theta}_{t2}-\dot{z}_{w3} ) \nonumber \\
&-l_w k_p(z_{t2}+l_w\theta_{t2}-z_{w4})-l_w c_p(\dot{z}_{t2}+l_w\dot{\theta}_{t2}-\dot{z}_{w4}),
\label{eq:bogie4}
\end{align}
where $I_t$ is the boige pitch inertia, $\theta_{t1}$ and $\theta_{t2}$ are the pitch angles of the first and the second bogie respectively, $l_w$ is a half of the bogie wheel base (Figure \ref{fig:mdof_model}), and $z_{w1},\ldots,z_{w4}$ are the vertical track irregularities experienced by the four wheels. These irregularities are considered to be the inputs to the system.

Further by substituting equations (\ref{eq:force1_2}) and (\ref{eq:force2_2}) into (\ref{eq:carbody_modes1})-(\ref{eq:higher_order_modes}) and then rewriting these equations together with (\ref{eq:bogie1})-(\ref{eq:bogie4}), the following matrix equation can be obtained
\begin{align}
\label{eq:mat_form}
\mathbf{M}\ddot{y} + \mathbf{C}\dot{y} + \mathbf{K}y = \mathbf{D_w}z_w + \mathbf{D_{dw}}\dot{z}_w,
\end{align}
where $y$ is a vector that contains all unknown variables 
\begin{equation*}
y = [z_b(t), \theta_b(t), q_3(t),\ldots,q_n(t),z_{t1}(t),z_{t2}(t),\theta_{t1}(t),\theta_{t2}(2)]^T,
\end{equation*}
and $z_w$ is a vector of input variables
\begin{equation*}
z_w = [z_{w1},z_{w2},z_{w3},z_{w4}]^T
\end{equation*}
In (\ref{eq:mat_form}) $\mathbf{M}$, $\mathbf{C}$, $\mathbf{K}$ are the inertia, damping, and stiffness matrices respectively, $\mathbf{D_w}$, $\mathbf{D_{dw}}$ are the track displacement and the velocity input matrices. These matrices contain the coefficients that appear next to the corresponding variables with same order of derivatives in equations (\ref{eq:carbody_modes1})-(\ref{eq:higher_order_modes}) and (\ref{eq:bogie1})-(\ref{eq:bogie4}).

In order to analyze the frequency characteristics of the carbody vibrations, the transfer function can be obtain by taking the Laplace transform of both sides of the equation in (\ref{eq:mat_form}) 
\begin{align}
\mathbf{M}&\mathcal{L}\left\{\ddot{y}\right\} + \mathbf{C}\mathcal{L}\left\{\dot{y}\right\} + \mathbf{K}\mathcal{L}\left\{y\right\} = \mathbf{D_w}\mathcal{L}\left\{z_w \right\} + \mathbf{D_{dw}}\mathcal{L}\{\dot{z}_w\mathcal\} \nonumber\\
\mathbf{M}&s^2\mathcal{Y}(s) + \mathbf{C}s\mathcal{Y}(s) + \mathbf{K}\mathcal{Y}(s) = \mathbf{D_w}s\mathcal{Z}_w(s) + \mathbf{D_{dw}}\mathcal{Z}_w(s)\nonumber\\
\mathcal{Y}(s)& \left[\mathbf{M}s^2+ \mathbf{C}s + \mathbf{K}\right] = \mathcal{Z}_w(s)\left[\mathbf{D_w}s + \mathbf{D_{dw}}\right]\nonumber\\
\mathcal{H}(s)& = \frac{\mathcal{Z}_w(s)}{\mathcal{Y}(s)}=\left[\mathbf{M}s^2+ \mathbf{C}s + \mathbf{K}\right]^{-1}\left[\mathbf{D_w}s + \mathbf{D_{dw}}\right]
\end{align}
where $\mathcal{H}(s)$ is a system transfer function, and $s$ is a complex number frequency parameter.
